# Supplementary material for: Graph-neural-network predictions of solid-state NMR parameters from spherical tensor decomposition
Source: arXiv:2412.15063 ancillary file (2024-12-19)
Supplement: Supplementary file 1 [file SI.pdf]

# Supplemental Materials for "Graph-neural-network predictions of solid-state NMR parameters from spherical tensor decomposition"

Chiheb Ben Mahmoud,[1, a)] Louise A. M. Rosset,[1] Jonathan R. Yates,[2] and Volker L. Deringer[1]

[1)] *Inorganic Chemistry Laboratory, Department of Chemistry, University of Oxford, Oxford OX1 3QR, United Kingdom*

[2)] *Department of Materials, University of Oxford, Oxford OX1 3PH, United Kingdom*

(Dated: December 11, 2024)

[a)] Electronic mail: chiheb.benmahmoud@chem.ox.ac.uk

## I. NMR PARAMETERS

In the main text, we discuss a few conventions that the NMR community uses to report the skewness of the magnetic shielding (MS) tensor, such as the Maryland convention and the Haeberlen convention. Both conventions rely on the eigenvalues of the MS tensor but differ in their ordering. The Maryland convention uses a standard ordering: $\sigma_{11} \geq \sigma_{22} \geq \sigma_{33}$, while the Haeberlen convention uses, in addition to the isotropic value $\sigma_{\text{iso}}$, the following ordering: $|\sigma_{\text{ZZ}} - \sigma_{\text{iso}}| \geq |\sigma_{\text{XX}} - \sigma_{\text{iso}}| \geq |\sigma_{\text{YY}} - \sigma_{\text{iso}}|$. In Table S1, we report the full definitions of these conventions using the specified orderings of the eigenvalues of the MS tensor.

Table S1: Definition of the parameters of the Maryland and Haeberlen conventions for the magnetic shielding tensor.

| convention | parameter 1 | parameter 2 |
|---|---|---|
| Maryland | span $\Omega = \sigma_{11} - \sigma_{33}$ | skew $\kappa = \frac{3}{2}(\sigma_{\text{iso}} - \sigma_{22})/\Omega$ |
| Haeberlen | anisotropy $\zeta = \sigma_{\text{iso}} - \sigma_{\text{ZZ}}$ | asymmetry $\eta = (\sigma_{\text{YY}} - \sigma_{\text{XX}})/\zeta$ |

## II. HYPERPARAMETERS OF THE NEQUIP MODELS

In Table S2, we report the results of the hyperparameter Bayesian optimization conducted using XPOT. In particular, the Bayesian optimization is conducted over categories for the following hyperparameters:

- `invariant_layers:` [1, 2, 3, 4]
- `invariant_neurons:` [16, 32, 64, 128]
- `num_layers:` [2, 3, 4, 5, 6]

In the case `features_irreps_hidden`, the optimization of the ISD models looped over :

$$\begin{aligned}
&[16\text{x0e} + 16\text{x1e} + 16\text{x2e} + 16\text{x0o} + 16\text{x1o} + 16\text{x2o},\\
&32\text{x0e} + 32\text{x1e} + 32\text{x2e} + 32\text{x0o} + 32\text{x1o} + 32\text{x2o},\\
&64\text{x0e} + 64\text{x1e} + 64\text{x2e} + 64\text{x0o} + 64\text{x1o} + 64\text{x2o},\\
&128\text{x0e} + 128\text{x1e} + 128\text{x2e} + 128\text{x0o} + 128\text{x1o} + 128\text{x2o}].
\end{aligned}$$

The optimization of the TP models looped initially over

$$\begin{aligned}
&[32\text{x0e} + 32\text{x1o},\\
&64\text{x0e} + 64\text{x1o},\\
&128\text{x0e} + 128\text{x1o},\\
&32\text{x0e} + 32\text{x1o} + 32\text{x2e},\\
&64\text{x0e} + 64\text{x1o} + 64\text{x2e},\\
&128\text{x0e} + 128\text{x1o} + 128\text{x2e},\\
&16\text{x0e} + 16\text{x1o},\\
&16\text{x0e} + 16\text{x1o} + 16\text{x2e}]
\end{aligned}$$

for a model targeting TPs of order $\ell = 2$. We find the model using 64x0e+64x1o+64x2e to perform the best in the small test set. Then, we adjust the maximum of the features to match the order of the tensors involved in the TP, for example if we want to use $\ell = 3$ for tensors involved in the TP, then we choose 64x0e+64x1o+64x2e+64x3o.

## III. RAW VALUES OF THE MS TENSOR TEST ERRORS

In Table S3, we show the root mean square errors (RMSE) evaluated on the a-$SiO_2$ test set for MS tensor-derived properties from the irreducible spherical decomposition (ISD) and the tensor product (TP) models. We also show the standard deviation (STD) of the quantum-mechanical (QM) target.

Table S2: Relevant hyperparameters of the irreducible spherical decomposition (ISD) and tensor product (TP) models obtained with to XPOT.

| | ISD-based model | tensor-product-based model |
|---|---|---|
| `r_max` (Å) | 5.53 | 4.31 |
| `invariant_layers` | 1 | 2 |
| `invariant_neurons` | 64 | 128 |
| `num_layers` | 6 | 4 |
| `features_irreps_hidden` | 128x0e+128x1e+128x2e+128x0o+128x1o+128x2o | 64x0e+64x1o+64x2e+64x3o+64x4e |

Table S3: Overview of errors and the standard deviation of irreducible tenors of MS and other derived quantities of silicon and oxygen atoms from the ISD and tensor product models in the a-$SiO_2$ test set.

| | silicon | | | oxygen | | |
|---|---|---|---|---|---|---|
| | ISD-RMSE | TP-RMSE | QM-STD | ISD-RMSE | TP-RMSE | QM-STD |
| $\sigma^{(0)}$ (ppm) | 0.59 | 0.64 | 8.65 | 1.56 | 2.11 | 17.76 |
| $\sigma^{(1)}$ (ppm) | 0.61 | 0.84 | 8.58 | 0.80 | 0.97 | 3.06 |
| $\sigma^{(2)}$ (ppm) | 1.23 | 1.80 | 16.97 | 2.10 | 2.90 | 27.70 |
| $\eta_\sigma$ | 1.64 | 2.62 | 23.93 | 2.89 | 3.77 | 18.14 |
| $\zeta_\sigma$ | 0.08 | 0.09 | 0.24 | 0.06 | 0.08 | 0.22 |
| $\kappa_\sigma$ | 0.08 | 0.09 | 0.39 | 0.06 | 0.08 | 0.29 |
| $\Omega_\sigma$ (ppm) | 1.93 | 3.08 | 27.70 | 3.38 | 4.48 | 18.53 |
| $\alpha_\sigma$ (rad) | 0.10 | 0.11 | 0.46 | 0.15 | 0.19 | 0.45 |
| $\beta_\sigma$ (rad) | 0.05 | 0.06 | 0.38 | 0.04 | 0.04 | 0.38 |
| $\gamma_\sigma$ (rad) | 0.10 | 0.11 | 0.91 | 0.07 | 0.08 | 0.91 |

## IV. TEST ERRORS OF THE EFG TENSOR

In Table S4, we show the RMSE, relative RMSE (%RMSE), and the QM standard deviation of the EFG-derived properties evaluated on the a-$SiO_2$ test set.

Table S4: Overview of errors and the standard deviation of irreducible tensors of MS and other derived quantities of silicon and oxygen atoms from the ISD and tensor product models in the a-$SiO_2$ test set.

| | silicon | | | oxygen | | |
|---|---|---|---|---|---|---|
| | RMSE | %RMSE | QM-STD | RMSE | %RMSE | QM-STD |
| $V^{(2)}$ | 0.004 (a.u.) | 2.01 | 0.20 (a.u.) | 0.010 (a.u.) | 1.84 | 0.55 (a.u.) |
| $V_{zz}$ | 0.051 (a.u.) | 14.81 | 0.35 (a.u.) | 0.057 (a.u.) | 21.64 | 0.26 (a.u.) |
| $\eta_Q$ | 0.005 | 2.39 | 0.23 | 0.014 | 6.53 | 0.21 |
| $\zeta_Q$ | 0.019 | 7.74 | 0.24 | 0.014 | 7.00 | 0.19 |
| $\kappa_Q$ | 0.018 | 4.21 | 0.42 | 0.015 | 6.38 | 0.23 |
| $\Omega_Q$ | 0.006 | 2.36 | 0.27 | 0.015 | 7.78 | 0.20 |
| $\alpha_Q$ | 0.056 (rad) | 12.35 | 0.46 (rad) | 0.062 (rad) | 13.54 | 0.46 (rad) |
| $\beta_Q$ | 0.072 (rad) | 19.11 | 0.38 (rad) | 0.023 (rad) | 6.06 | 0.38 (rad) |
| $\gamma_Q$ | 0.104 (rad) | 11.46 | 0.91 (rad) | 0.042 (rad) | 4.66 | 0.91 (rad) |

## V. THE EFFECT OF THE INPUT HIDDEN FEATURES ON THE QUALITY OF THE PREDICTIONS

In Fig. S1, we show the effect of the maximum rank $\ell_{\max}$ of the hidden features of the ML model on the prediction quality of the MS tensor properties. We observe that the maximum rank of the features should at least match or exceed the rank of $\sigma^{(\ell)}$. In our dataset, we do not see any significant improvements beyond $\ell_{\max} = 2$ for the hidden features. A higher rank of hidden features translates to more fitting parameters and a more expressive model. It is possible that our dataset is too small to fully leverage the model parameters.

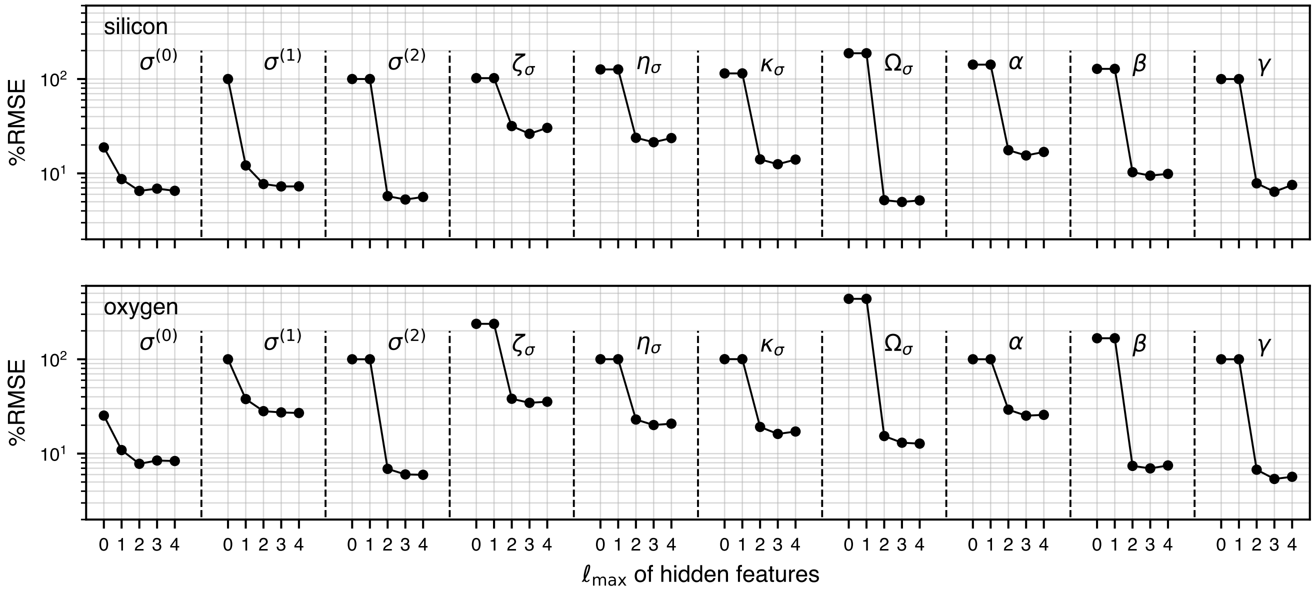


Figure S1: Effect of the max rank $\ell_{\max}$ of the hidden features on the properties of the chemical shielding ML models, evaluated using the irreducible spherical decomposition representation. Upper panel: silicon atoms; lower panel: oxygen atoms.

## VI. MS AND EFG TENSORS ERRORS IN A-SIO$_2$TRUCTURAL MODELS

In Table S5, we report the ML prediction errors for the irreducible tensors of the MS and EFG tensors in a dataset of three structural a-$SiO_2$ samples with densities $\rho = 2.2$, 2.4, and 2.6 g cm$^{-3}$. These configurations are obtained using the ML-based interatomic potential from Ref. S1. We show the %RMSE for the ISD and TP models for the MS, and only the ISD errors for the EFG. Additionally, we show the standard deviation of the target quantities for silicon and oxygen atoms.

Table S5: Overview of the standardized errors and the standard deviation of irreducible tensors of MS and EFG for silicon and oxygen atoms from the ISD and tensor product models in a dataset of three a-$SiO_2$ structural models.

| | silicon | | | oxygen | | |
|---|---|---|---|---|---|---|
| | ISD-%RMSE | TP-%RMSE | QM-STD | ISD-%RMSE | TP-%RMSE | QM-STD |
| $\sigma^{(0)}$ | 5.14 | 4.90 | 8.67 (ppm) | 7.60 | 7.93 | 13.07 (ppm) |
| $\sigma^{(1)}$ | 4.99 | 5.17 | 8.44 (ppm) | 18.41 | 20.15 | 2.41 (ppm) |
| $\sigma^{(2)}$ | 6.90 | 8.02 | 13.46 (ppm) | 5.46 | 7.17 | 25.49 (ppm) |
| $V^{(2)}$ | 2.17 | – | 0.16 (a.u.) | 1.72 | – | 0.51 (a.u.) |

## VII. MS AND EFG TENSORS ERRORS IN $SIO_2$ HYPOTHETICAL ZEOLITES

In Table S6, we report the ML prediction errors for the irreducible tensors of the MS and EFG tensors in a dataset of 50 $SiO_2$ hypothetical zeolites. We show the %RMSE for the ISD and TP models for the MS, and only the ISD errors for the EFG. Additionally, we show the standard deviation of the target quantities for silicon and oxygen atoms.

Table S6: Overview of the standardized errors and the standard deviation of irreducible tensors of MS and EFG of silicon and oxygen atoms from the ISD and TP models in a dataset of $SiO_2$ hypothetical zeolites.

| | silicon | | | oxygen | | |
|---|---|---|---|---|---|---|
| | ISD-%RMSE | TP-%RMSE | QM-STD | ISD-%RMSE | TP-%RMSE | QM-STD |
| $\sigma^{(0)}$ | 3.96 | 3.93 | 6.24 (ppm) | 9.78 | 9.48 | 5.67 (ppm) |
| $\sigma^{(1)}$ | 2.20 | 2.25 | 6.45 (ppm) | 25.4 | 32.37 | 0.63 (ppm) |
| $\sigma^{(2)}$ | 6.4 | 8.91 | 7.46 (ppm) | 2.60 | 3.28 | 30.82 (ppm) |
| $V^{(2)}$ | 4.06 | – | 0.06 (a.u.) | 1.54 | – | 0.52 (a.u.) |

## VIII. RING SIZE DISTRIBUTION IN THE TRAINING SET

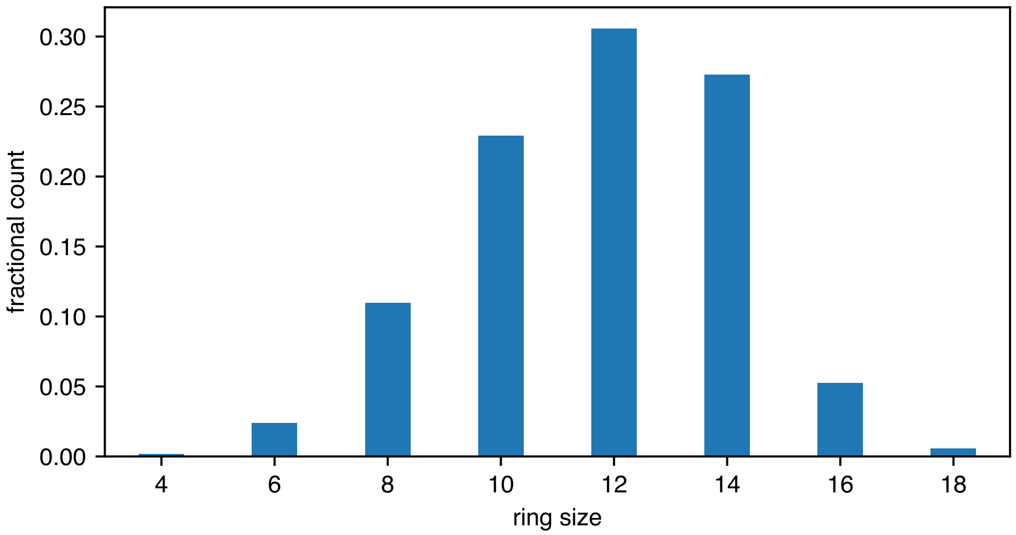


Figure S2: Distribution of ring sizes in the training set.

In Fig. S2, we report the ring-size distribution in the training set. The smallest ring contains 4 members, while the largest ring contains 18 members. Our extrapolation sets (structural models and zeolites) contain structures with ring sizes of up to 24 members.

## REFERENCES


[S1] L. C. Erhard, J. Rohrer, K. Albe, and V. L. Deringer, Nature Communications **15**, 1927 (2024).
